# Supplementary material for: CornerFormer: Boosting Corner Representation for Fine-Grained Structured Reconstruction
Source: arXiv:2304.07072 source file (2023-12-12)
Supplement: Supplementary file 1 [file table_edge_decoder_supp.tex]

\begin{table}[!h]
    \centering
    \small
    \caption{
    }
    % \resizebox{\textwidth}{!}
    {
        \tabcolsep 3pt
	    \begin{tabu}{@{\;} lccccc@{\;}}
	        \addlinespace
	        \toprule
	        % {Eval Type } & \multicolumn{3}{c}{Edge} &  \multicolumn{3}{c}{Region} \\
	        % \cmidrule(lr){2-4}\cmidrule(lr){5-7}
	        Structure  &Output& Corner & Edge &Region & Param(M) \\
                \midrule
                \multirow{2}{*}{Structure$(a)$}  & $O_{boost}$ &  88.5 & 78.3 & 69.8 & 50.70 &  
                &$O_{edge}$ &  88.5 & 78.3 & 69.9 & 50.70  \\
                \midrule
                \multirow{2}{*}{Structure$(b)$} 
                &$O_{boost}$ & 88.3 & 77.7 & 70.0 & 50.70 &
                & $O_{edge}$ & 88.4 & 78.3 & 71.3 & 50.70  \\
                \midrule
                \multirow{2}{*}{Structure$(c)$}  & $O_{boost}$ & 88.5 & 78.5 & 71.4 & 46.97 &
                & $O_{edge}$ & 89.0 & 79.2 & 71.9 & 46.97  \\
    	    \bottomrule
	    \end{tabu}
	}
    \label{tab:structure}
\end{table}
